# Supplementary material for: KI-GAN: Knowledge-Informed Generative Adversarial Networks for Enhanced Multi-Vehicle Trajectory Forecasting at Signalized Intersections
Source: arXiv:2404.11181 source file (2024-04-19)
Supplement: Supplementary file 1 [file X_suppl.tex]

\clearpage
\setcounter{page}{1}
\maketitlesupplementary
